# Supplementary material for: A coarse-to-fine framework for unsupervised multi-contrast MR image deformable registration with dual consistency constraint
Source: arXiv:2008.01896 source file (2021-02-16)
Supplement: Supplementary file 1 [file supplementary.tex]

%\subsection{Network architecture details}
%Here we describe the full network architecture used in our experiments. Let Ck-s denote a 3D convolution layer with $k$ filters and a stride of $s$. All convolutions use a kernel size of $3$, and are followed by a LeakyReLU layer with $\alpha=0.2$. We use the notation $c_i$ to denote the output of each convolution in the encoder. Let U represent a 3D upsampling layer, and A$c_i$ denote concatenation with the volume $c_i$ from the encoder.\\
%
%\noindent Encoder: C16-2 ($c_1$), C32-2 ($c_2$), C32-2 ($c_3$), C32-2 ($c_4$)\\
%Decoder: C32, U, A$c_3$, C32, U, A$c_2$, C32, U, A$c_1$, C32, C32, U, C16, C16
\begin{figure}[b]\setlength{\hfuzz}{1.1\columnwidth}
\hspace{-250pt}
\begin{minipage}{\textwidth}
%\ttfamily 

%\begin{figure*}[h!]
	\begin{center}
		\includegraphics[width=0.7\linewidth]{figures/brains_remainder_withflows.jpg}
	\end{center}
	\caption{\color{blue}Example atlas-based VoxelMorph flow fields $\bphi$ (columns 4-5) extracted by registering the moving image (column 1) to the fixed image (column 2). The warped image $\bmoving \circ \biphi$ is shown in column 3. 
	}
	\label{fig:sup-brains}
%\end{figure*}
\end{minipage}
\end{figure}

\begin{figure*}[h!]
	\begin{center}
	\begin{subfigure}[b]{0.33\linewidth}
		\includegraphics[width=\linewidth]{figures/brains_hippo_0_01_samples_remainder_withflows.jpg}
	\end{subfigure} 
	~
		\begin{subfigure}[b]{0.33\linewidth}
		\includegraphics[width=\linewidth]{figures/brains_hippo_inf_samples_remainder_withflows.jpg}
	\end{subfigure}
		\end{center}
	\caption{\color{blue}Auxiliary data experiment where the left and right hippocampus labels are observed at train time. We show the moving image, fixed image and warped image (columns 1-3) with the observed labels overlaid, and the resulting deformation fields (columns 4-5). We use the optimal $\gamma=0.01$ (left) and the extreme $\gamma=\infty$ (right).  
	}
	\label{fig:supp_labels_hippo}
\end{figure*}

\begin{figure*}[h!]
	\begin{center}
	\begin{subfigure}[b]{0.33\linewidth}
		\includegraphics[width=\linewidth]{figures/brains_halfout_0_01_samples_remainder_withflows.jpg}
	\end{subfigure} 
	~
		\begin{subfigure}[b]{0.33\linewidth}
		\includegraphics[width=\linewidth]{figures/brains_halfout_inf_samples_remainder_withflows.jpg}
	\end{subfigure}
		\end{center}
	\caption{\color{blue}Auxiliary data experiment where a random half of the labels are observed at train time. We show the moving image, fixed image and warped image (columns 1-3) with the observed labels overlaid, and the resulting deformation fields (columns 4-5). We use the optimal $\gamma=0.01$ (left) and the extreme $\gamma=\infty$ (right).  
	}
	\label{fig:supp_labels_half}
\end{figure*}

\begin{figure*}[h!]
	\begin{center}
	\begin{subfigure}[b]{0.33\linewidth}
		\includegraphics[width=\linewidth]{figures/brains_all_0_01_samples_remainder_withflows.jpg}
	\end{subfigure} 
	~
		\begin{subfigure}[b]{0.33\linewidth}
		\includegraphics[width=\linewidth]{figures/brains_all_inf_samples_remainder_withflows.jpg}
	\end{subfigure}
		\end{center}
	\caption{\color{blue}Auxiliary data experiment where all labels are observed at train time. We show the moving image, fixed image and warped image (columns 1-3) with the observed labels overlaid, and the resulting deformation fields (columns 4-5). We use the optimal $\gamma=0.01$ (left) and the extreme $\gamma=\infty$ (right).  
	}
	\label{fig:supp_labels_all}
\end{figure*}

\begin{figure*}[h!]
	\begin{center}
	\begin{subfigure}[b]{0.33\linewidth}
		\includegraphics[width=\linewidth]{figures/brains_merge_0_01_samples_remainder_withflows.jpg}
	\end{subfigure} 
	~
		\begin{subfigure}[b]{0.33\linewidth}
		\includegraphics[width=\linewidth]{figures/brains_merge_inf_samples_remainder_withflows.jpg}
	\end{subfigure}
		\end{center}
	\caption{\color{blue}Auxiliary data experiment where coarse labels are observed at train time. We show the moving image, fixed image and warped image (columns 1-3) with the observed labels overlaid, and the resulting deformation fields (columns 4-5). We use the optimal $\gamma=0.01$ (left) and the extreme $\gamma=\infty$ (right).  
	}
	\label{fig:supp_labels_coarse}
\end{figure*}
